# Supplementary material for: Ternary Alkali Metal Copper Chalcogenides ACuX (A= Na, K and X= S, Se, Te): Promising Candidate for Solar Harvesting Applications
Source: arXiv:2312.16063 ancillary file (2023-12-26)
Supplement: Supplementary file 1 [file Supplement.pdf]

## Supplementary Information

### Ternary Alkali Metal Copper Chalcogenides ACuX (A= Na, K and X= S, Se, Te): Promising Candidate for Solar Harvesting Applications

Gurudayal Behera,<sup>1</sup> Surabhi Suresh Nair,<sup>2</sup> Nirpendra Singh,<sup>2</sup> K. R. Balasubramaniam,<sup>1,\*</sup> and Aftab Alam<sup>3,†</sup>

<sup>1</sup>*Department of Energy Science and Engineering, IIT Bombay, Powai, Mumbai 400076, India*

<sup>2</sup>*Department of Physics, Khalifa University of Science and Technology, Abu Dhabi 127788, United Arab Emirates*

<sup>3</sup>*Department of Physics, Indian Institute of Technology, Bombay, Powai, Mumbai 400076, India*

Here, we provide further theoretical backgrounds on optical properties calculations, formation energies for different space group lattices of ACuX compound and their phonon dispersion plots for the energetically most stable structures, SOC band structure plots, orbital projected DOS for CBM side of ACuX and absorption spectra of orthorhombic structures along the yy-polarization direction.

#### I. Optical properties and Spectroscopic Limited maximum efficiency (SLME)

##### A. Optical properties

The frequency dependent dielectric constants were calculated using DFT within the independent particle approximation (IPA)[1–3] method as implemented in VASP. The complex dielectric function can be written as,

$$\varepsilon(\omega) = \varepsilon_1(\omega) + i\varepsilon_2(\omega) \quad (1)$$

where  $\varepsilon_1(\omega)$  and  $\varepsilon_2(\omega)$  are the real and imaginary parts of the complex dielectric constants, respectively. The  $\varepsilon_2(\omega)$  is determined by a summation over the electronic states using the following equation [1],

$$\varepsilon_2^{\alpha\beta}(\omega) = \frac{4\pi e^2}{\Omega} \lim_{q \rightarrow 0} \frac{1}{q^2} \sum_{c,v,k} 2\omega_k \delta(\varepsilon_{ck} - \varepsilon_{vk} - \omega) \langle u_{ck+e_{\alpha}q} | u_{vk} \rangle \langle u_{vk} | u_{ck+e_{\beta}q} \rangle \quad (2)$$

where  $\Omega$  is the crystal volume and the indices  $\alpha$  and  $\beta$  represent the cartesian components of the unit vectors  $e_{\alpha}$  and  $e_{\beta}$ .  $c$  and  $v$  refer to conduction and valence band states, respectively, and  $u_{ck}$  is the periodic cell part of the orbitals at the  $k$ -points. Now real part of the dielectric tensor is obtained by the well-known Kramers-Kronig relation[4],

$$\varepsilon_1^{\alpha\beta}(\omega) = 1 + \frac{2}{\pi} P \int_0^{\infty} \frac{\varepsilon_2^{\alpha\beta}(\omega') \omega'}{\omega'^2 - \omega^2 + i\eta} d\omega' \quad (3)$$

where  $P$  is the principle value of the integral. We can calculate the absorption coefficient ( $\alpha$ ) using these dielectric tensors by the following expression:

$$\alpha(E) = \frac{\sqrt{2}\omega}{c} \left[ \sqrt{\varepsilon_1^2(\omega) + \varepsilon_2^2(\omega)} - \varepsilon_1 \right] \quad (4)$$

where  $E$  is the incident photon energy,  $\omega$  is the angular frequency related to photon energy via  $E = \hbar\omega$  ( $\hbar$  is the reduced Planck's constant), and  $c$  is the speed of light in vacuum, respectively.

##### B. Spectroscopic Limited Maximum Efficiency (SLME)

Spectroscopic Limited Maximum Efficiency (SLME) is an improved version of the Shockley-Queisser (SQ) efficiency limit. This was proposed by Yu *et al.*[5] in 2012 to evaluate the maximum possible efficiency for a solar absorber

---

\* bala.ramanathan@iitb.ac.in

† aftab@iitb.ac.in

thin-film material theoretically. According to the SQ limit, the power conversion efficiency of a photovoltaic cell is defined by,

$$\eta = \frac{P_{max}}{P_{input}} \quad (5)$$

where  $P_{input}$  is the input power density of the incident solar spectrum and  $P_{max}$  is the maximum possible output power density for a material. The  $P_{max}$  can be found by maximizing the power density by numerically maximizing the product of current density (J) and voltage (V) from the J-V characteristic plot of an illuminated solar cell. Now, J can be defined as,

$$J = J_{sc} - J_0(e^{\frac{eV}{k_B T}} - 1) \quad (6)$$

where  $J_{sc}$  is the short-circuit current density and  $J_0$  is total recombination current density,  $k_B$  is the Boltzmann constant and T is the temperature.  $J_{sc}$  can be defined as,

$$J_{sc} = e \int_0^\infty a(E) I_{sun}(E) dE \quad (7)$$

Here e is the electronic charge,  $a(E)$  is absorptivity, and  $I_{sun}(E)$  is the photon flux from the incident solar spectrum at standard AM1.5G solar spectrum at 298 K.

As we know, SQ efficiency only depends on the band gap, irrespective of the material. However, SLME includes two parameters that are very closely related to material properties *i.e.*, (i) the nature of the band gap and (ii) optical absorption spectra. So far, the reason behind most of the indirect band gap materials failing as solar absorbers because of their poor absorption as well as a much higher recombination rate than a direct band gap material. Hence, the carrier recombination rate can be roughly divided into two parts (i) radiative and (ii) non-radiative. Hence,  $J_0$  can be defined as  $J_0 = J_0^r + J_0^{nr}$  ( $J_0^r$  for radiative and  $J_0^{nr}$  for non-radiative recombination current density, respectively). For the direct band gap materials the first part is dominant, the second being negligible. In contrast, the non-radiative recombination rises to prominence as the indirect nature of the band gap increases. In SLME calculation, the non-radiative part is taken into account and proposes a new parameter  $f_r$ , which is defined as,

$$f_r = e^{\frac{E_g^{da} - E_g}{k_B T}} \quad (8)$$

Here  $E_g^{da}$  is the direct band gap allowing direct optical transition, and  $E_g$  is the electronic band gap. For a direct band gap material  $f_r = 1$ , which makes the non-radiative loss zero. So using the factor  $f_r$ ,  $J_0^r$  can be defined as,

$$J_0 = \frac{J_0^r}{f_r} \quad (9)$$

According to the principle of detailed balance, emission, and absorption rates through cell surfaces must be equal in equilibrium in the dark. Hence  $J_0^r$  can be calculated from the rate at which black-body photons from the surrounding thermal bath are absorbed through the front surface[6],

$$J_0^r = e\pi \int_0^\infty a(E) I_{bb}(E, T) dE \quad (10)$$

where  $I_{bb}$  is the black-body spectrum at temperature T. Therefore, we need to simulate the band structure to find the band gap value with nature and absorption spectra to calculate the SLME of a specific material at a certain temperature and film thickness.

## II. Prototype crystal structures, Formation energies, and phonon dispersion for ACuX compounds in different space groups

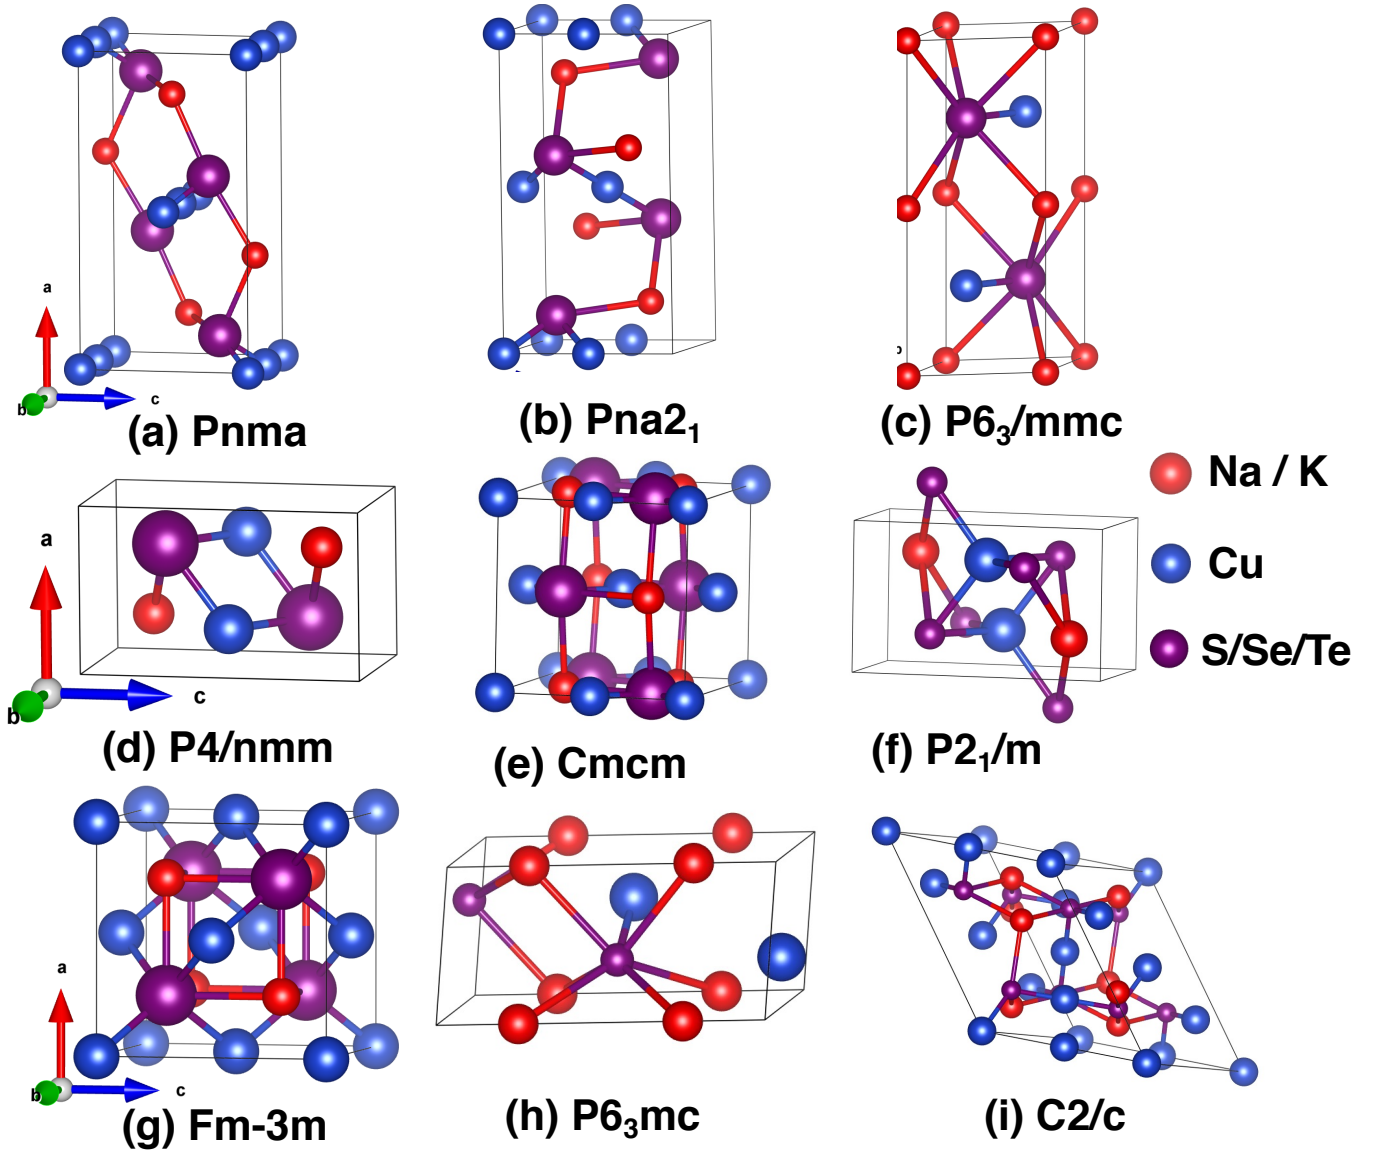

FIG. S1. Nine prototype crystal structures which has competing formation enthalpies for  $ACuX$  ( $A=Na,K$ ;  $X= S, Se, Te$ ) compounds.

TABLE S1. Optimized lattice constants ( $a, b, c$ ) (in  $\text{\AA}$ ) and the corresponding formation energy ( $\Delta E_F$  in eV/atom) for  $NaCuS$  in different space groups.  $\Delta$  is the energy of  $NaCuS$  with respect to the lowest energy structures.

| Space group          | Optimized<br>lattice parameters ( $\text{\AA}$ ) | No. of atoms<br>in unitcell | Formation energy<br>$\Delta E_F$ (eV/atom) | $\Delta = \Delta E_F - \Delta E_{Fmin}$<br>(meV/atom) |
|----------------------|--------------------------------------------------|-----------------------------|--------------------------------------------|-------------------------------------------------------|
| Pnma                 | $a = 8.17, b = 3.93, c = 6.80$                   | 12                          | -0.687                                     | 21                                                    |
| Pna2 <sub>1</sub>    | $a = 9.48, b = 5.65, c = 5.13$                   | 12                          | -0.708                                     | 0                                                     |
| P6 <sub>3</sub> /mmc | $a = 3.93, c = 8.17$                             | 6                           | -0.687                                     | 21                                                    |
| P4/nmm               | $a = 3.92, c = 6.63$                             | 6                           | -0.646                                     | 62                                                    |
| Cmcm                 | $a = 3.93, b = 6.80, c = 8.17$                   | 12                          | -0.687                                     | 21                                                    |
| P2 <sub>1</sub> /m   | $a = 3.90, b = 3.91, c = 6.62$                   | 6                           | -0.646                                     | 62                                                    |
| F43m                 | $a = 5.9$                                        | 12                          | -0.396                                     | 312                                                   |
| P6 <sub>3</sub> mc   | $a = 3.93, b = 8.18$                             | 6                           | -0.687                                     | 21                                                    |
| C2/c                 | $a = 8.99, b = 9.75, c = 7.31$                   | 24                          | -0.646                                     | 62                                                    |

TABLE S2. Optimized lattice constants (a, b, c) (in Å) and the corresponding formation energy ( $\Delta E_F$  in eV/atom) for NaCuSe in different space groups.  $\Delta$  is the energy of NaCuSe with respect to the lowest energy structures.

| Space group          | Optimized<br>lattice parameters (Å) | No. of atoms<br>in unitcell | Formation energy<br>$\Delta E_F$ (eV/atom) | $\Delta = \Delta E_F - \Delta E_{Fmin}$<br>(meV/atom) |
|----------------------|-------------------------------------|-----------------------------|--------------------------------------------|-------------------------------------------------------|
| Pnma                 | a=9.97, b= 5.24, c= 5.87            | 12                          | -0.629                                     | 7                                                     |
| Pna2 <sub>1</sub>    | a=11.02, b= 6.47, c= 5.47           | 12                          | -0.629                                     | 7                                                     |
| P6 <sub>3</sub> /mmc | a=4.14, c=8.34                      | 6                           | -0.637                                     | 0                                                     |
| P4/nmm               | a= 4.09, b= 6.87                    | 6                           | -0.617                                     | 20                                                    |
| Cmcm                 | a= 5.94, b= 7.60, c= 5.96           | 12                          | -0.575                                     | 62                                                    |
| P2 <sub>1</sub> /m   | a= 4.08, b= 4.09, c=6.86            | 6                           | -0.617                                     | 20                                                    |
| F43m                 | a= 6.12                             | 12                          | -0.453                                     | 184                                                   |
| P6 <sub>3</sub> mc   | a= 4.13, b= 8.45                    | 6                           | -0.627                                     | 10                                                    |
| C2/c                 | a= 9.44, b=10.33, c=7.61            | 24                          | -0.560                                     | 77                                                    |

TABLE S3. Optimized lattice constants (a, b, c) (in Å) and the corresponding formation energy ( $\Delta E_F$  in eV/atom) for NaCuTe in different space groups.  $\Delta$  is the energy of KCuTe with respect to the lowest energy structures.

| Space group          | Optimized<br>lattice parameters (Å) | No. of atoms<br>in unitcell | Formation energy<br>$\Delta E_F$ (eV/atom) | $\Delta = \Delta E_F - \Delta E_{Fmin}$<br>(meV/atom) |
|----------------------|-------------------------------------|-----------------------------|--------------------------------------------|-------------------------------------------------------|
| Pnma                 | a= 8.67, c= 4.42, c= 7.66           | 12                          | -0.505                                     | 5                                                     |
| Pna2 <sub>1</sub>    | a= 11.20, b= 5.608, c=5.38          | 12                          | -0.443                                     | 67                                                    |
| P6 <sub>3</sub> /mmc | a= 4.42, c= 8.69                    | 6                           | -0.510                                     | 0                                                     |
| P4/nmm               | a= 4.39, c= 7.13                    | 6                           | -0.493                                     | 17                                                    |
| Cmcm                 | a= 6.29, b= 7.86, c= 6.57           | 12                          | -0.397                                     | 113                                                   |
| P2 <sub>1</sub> /m   | a= 3.39, b= 4.38, c= 7.11           | 6                           | -0.493                                     | 17                                                    |
| F43m                 | a= 6.44                             | 12                          | -0.431                                     | 79                                                    |
| P6 <sub>3</sub> mc   | a= 4.42, c= 8.69                    | 6                           | -0.490                                     | 20                                                    |
| C2/c                 | a= 10.18, b=11.48, c= 7.96          | 24                          | -0.378                                     | 132                                                   |

TABLE S4. Optimized lattice constants (a, b, c) (in Å) and the corresponding formation energy ( $\Delta E_F$  in eV/atom) for KCuS in different space groups.  $\Delta$  is the energy of KCuS with respect to the lowest energy structures.

| Space group          | Optimized<br>lattice parameters (Å) | No. of atoms<br>in unitcell | Formation energy<br>$\Delta E_F$ (eV/atom) | $\Delta = \Delta E_F - \Delta E_{Fmin}$<br>(meV/atom) |
|----------------------|-------------------------------------|-----------------------------|--------------------------------------------|-------------------------------------------------------|
| Pnma                 | a= 10.97, b=5.34, c=6.30            | 12                          | -0.768                                     | 0                                                     |
| Pna2 <sub>1</sub>    | a= 10.88, b=6.34, c= 5.34           | 12                          | -0.768                                     | 0                                                     |
| P6 <sub>3</sub> /mmc | a= 4.01, c= 9.74                    | 6                           | -0.699                                     | 69                                                    |
| P4/nmm               | a= 4.14, c= 7.44                    | 6                           | -0.594                                     | 174                                                   |
| Cmcm                 | a= 6.34, b= 10.93, c= 5.74          | 12                          | -0.747                                     | 21                                                    |
| P2 <sub>1</sub> /m   | a= 6.19, b= 4.05, c= 6.88           | 6                           | -0.672                                     | 96                                                    |
| F43m                 | a= 6.42                             | 12                          | -0.144                                     | 624                                                   |
| P6 <sub>3</sub> mc   | a= 4.00, c= 4.72                    | 6                           | -0.699                                     | 69                                                    |
| C2/c                 | a= 9.81, b = 11.24, c= 7.56         | 24                          | -0.582                                     | 186                                                   |

TABLE S5. Optimized lattice constants (a, b, c) (in Å) and the corresponding formation energy ( $\Delta E_F$  in eV/atom) for KCuSe in different space groups.  $\Delta$  is the energy of KCuSe with respect to the lowest energy structures.

| Space group          | Optimized<br>lattice parameters (Å) | No. of atoms<br>in unitcell | Formation energy<br>$\Delta E_F$ (eV/atom) | $\Delta = \Delta E_F - \Delta E_{Fmin}$<br>(meV/atom) |
|----------------------|-------------------------------------|-----------------------------|--------------------------------------------|-------------------------------------------------------|
| Pnma                 | a=11.84, b= 5.43, c= 6.36           | 12                          | -0.697                                     | 0                                                     |
| Pna2 <sub>1</sub>    | a= 11.76, b= 6.40, c=5.44           | 12                          | -0.589                                     | 108                                                   |
| P6 <sub>3</sub> /mmc | a= 4.20, b =9.92                    | 6                           | -0.685                                     | 12                                                    |
| P4/nmm               | a= 4.34, c= 7.58                    | 6                           | -0.594                                     | 103                                                   |
| Cmcm                 | a= 6.71, b= 8.40, c= 6.29           | 12                          | -0.590                                     | 107                                                   |
| P2 <sub>1</sub> /m   | a= 4.33, b = 4.34, c= 7.56          | 6                           | -0.595                                     | 102                                                   |
| F43m                 | a= 6.62                             | 12                          | -0.247                                     | 450                                                   |
| P6 <sub>3</sub> mc   | a= 4.20, c= 9.90                    | 6                           | -0.685                                     | 12                                                    |
| C2/c                 | a= 10.17, b =12.03, c= 5.86         | 24                          | -0.540                                     | 157                                                   |

TABLE S6. Optimized lattice constants (a, b, c) (in Å) and the corresponding formation energy ( $\Delta E_F$  in eV/atom) for KCuTe in different space groups.  $\Delta$  is the energy of KCuTe with respect to the lowest energy structures.

| Space group          | Optimized<br>lattice parameters (Å) | No. of atoms<br>in unitcell | Formation energy<br>$\Delta E_F$ (eV/atom) | $\Delta = \Delta E_F - \Delta E_{Fmin}$<br>(meV/atom) |
|----------------------|-------------------------------------|-----------------------------|--------------------------------------------|-------------------------------------------------------|
| Pnma                 | a= 10.31, b= 4.48, c= 7.76          | 12                          | -0.595                                     | 0                                                     |
| Pna2 <sub>1</sub>    | a= 13.46, b= 5.23, c=5.47           | 12                          | -0.535                                     | 60                                                    |
| P6 <sub>3</sub> /mmc | a= 4.48, b= 10.31                   | 12                          | -0.595                                     | 0                                                     |
| P4/nmm               | a= 4.63, c= 7.83                    | 6                           | -0.511                                     | 84                                                    |
| Cmcm                 | a= 7.08, b= 8.50, c= 6.94           | 12                          | -0.504                                     | 91                                                    |
| P2 <sub>1</sub> /m   | a= 4.64, b= 6.61, c= 7.86           | 6                           | -0.512                                     | 83                                                    |
| F43m                 | a= 6.92                             | 12                          | -0.270                                     | 325                                                   |
| P6 <sub>3</sub> mc   | a= 4.48, c= 10.31                   | 24                          | -0.588                                     | 7                                                     |
| C2/c                 | a= 10.87, b= 13.18, c= 8.08         | 24                          | -0.417                                     | 178                                                   |

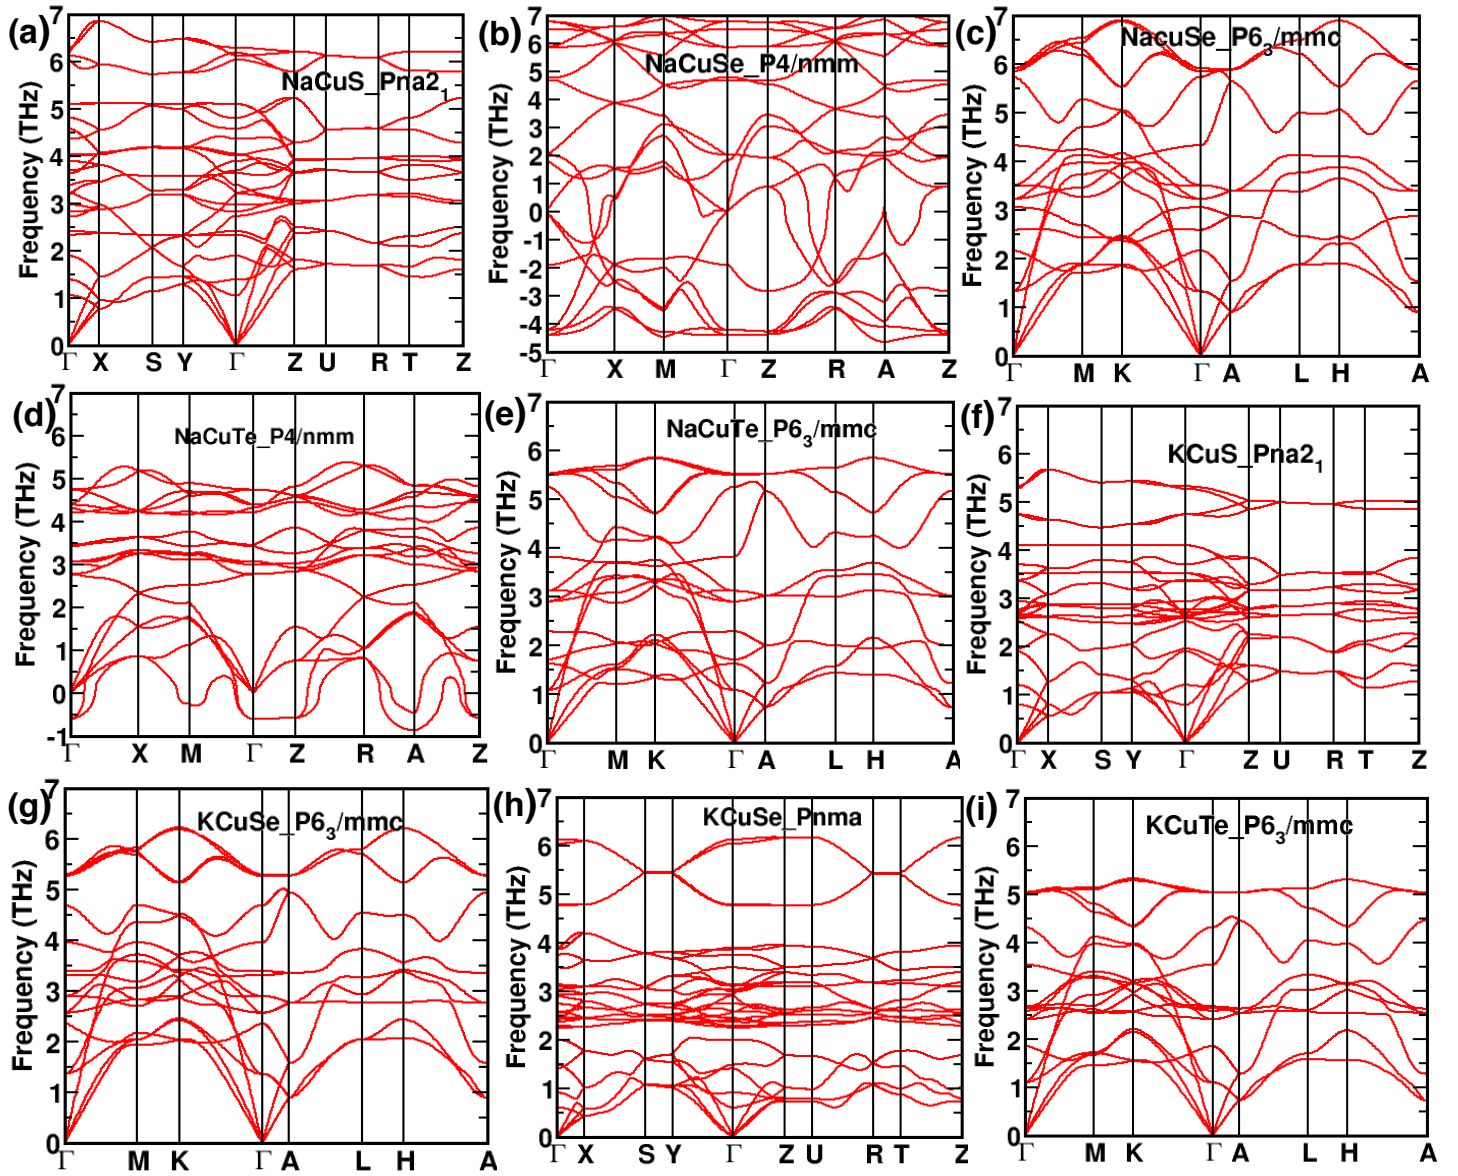

FIG. S2. Phonon dispersion of all ACuX compounds (A=K, Na; X=S, Se, Te) in their lowest energy structure and experimental reported ones.

### III. PBE vs. PBE+SOC band structures

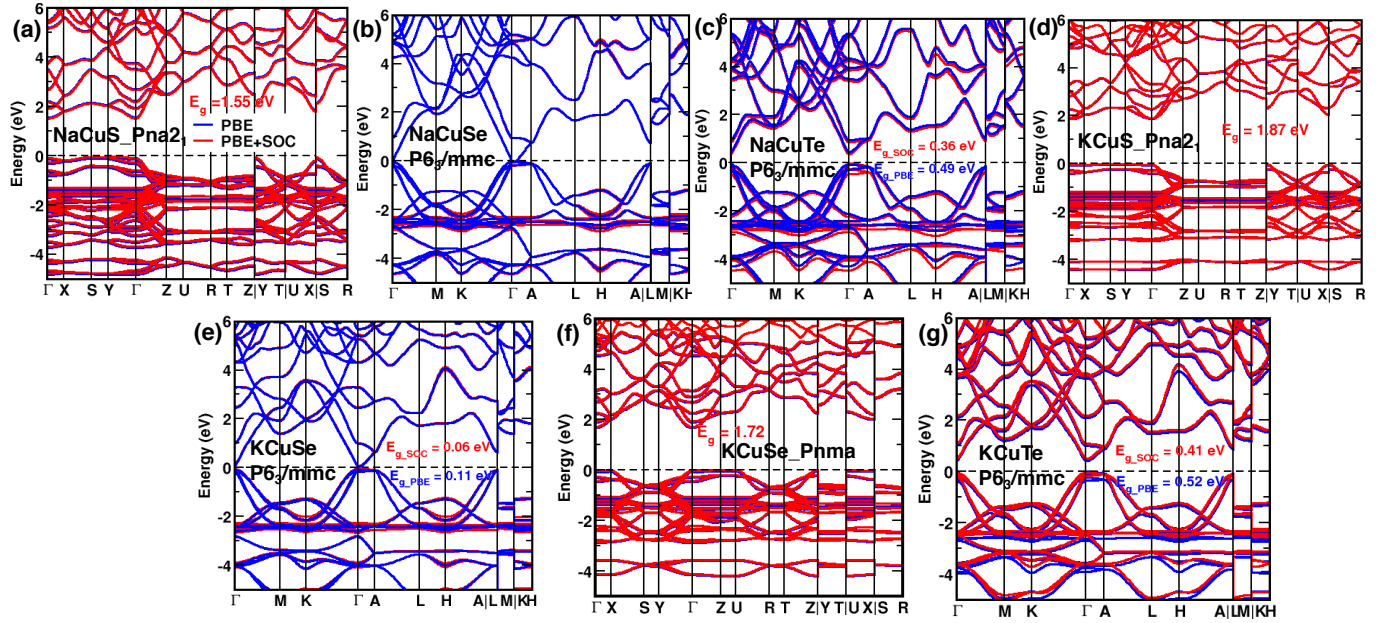

FIG. S3. Comparative band structures of different ACuX compounds using PBE functional with and without spin orbit coupling (SOC). Red/Blue curves indicate the band structures with/without SOC effect, respectively. Fermi level ( $E_f$ ) is set to zero, as shown by the horizontal dashed line.

### IV. Orbital projected density of states (DOS) above Fermi level for different ACuX compounds

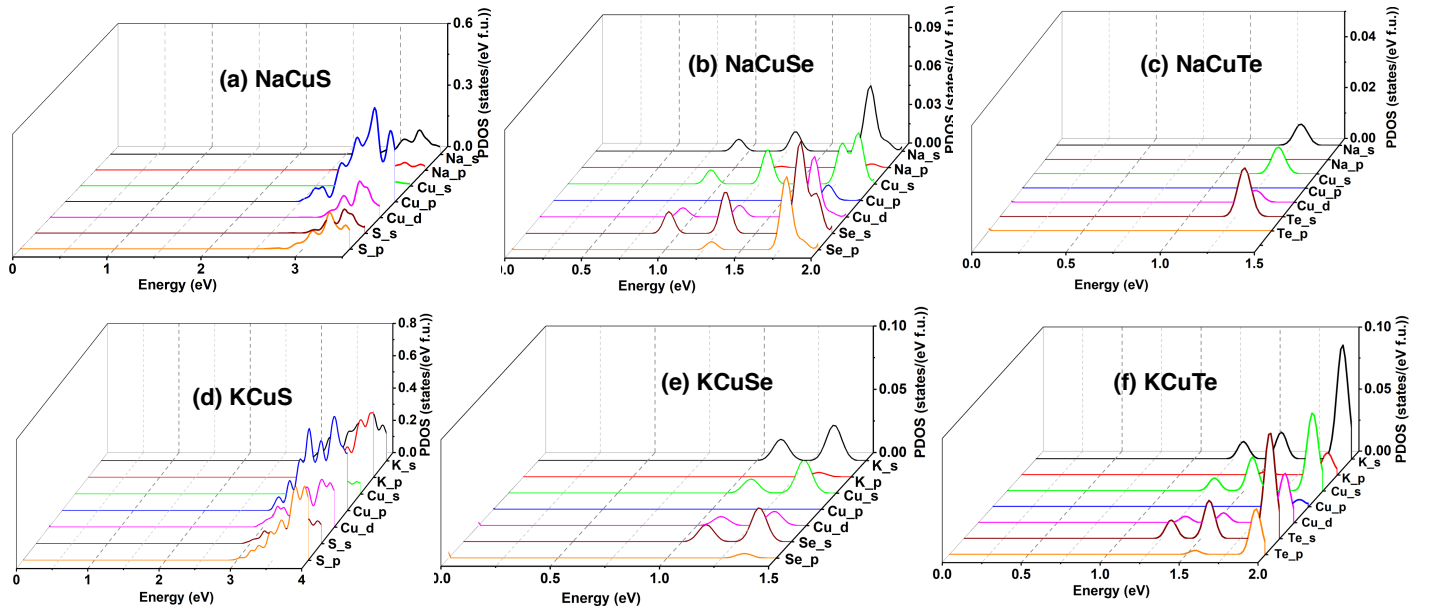

FIG. S4. Zoomed-in-view of orbital projected PDOS above  $E_f$  for (a,b,c) NaCuX and (d,e,f) KCuX (X=S/Se/Te) compounds, respectively.  $E_f$  is set at 0 eV.

# V. Absorption coefficient along y-polarization direction for orthorhombic ACuX compounds

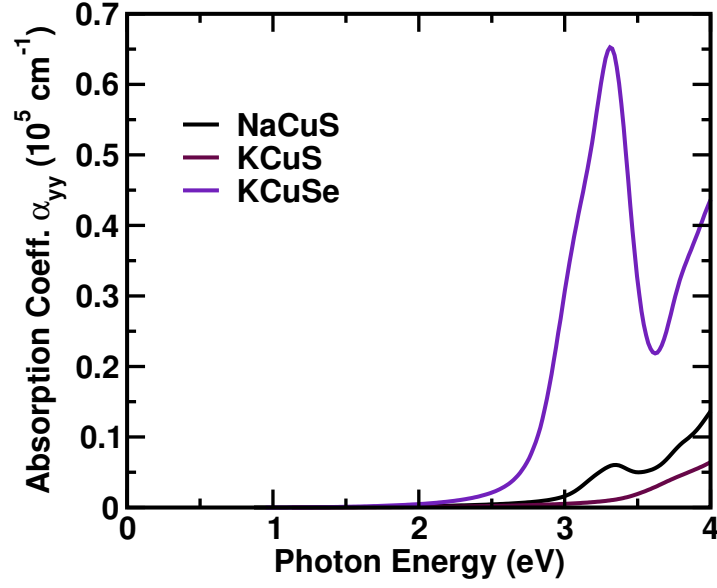

FIG. S5. Absorption spectra along y-polarization direction for selected compounds which stabilize in orthorhombic structures (where  $\alpha_{xx} \neq \alpha_{yy}$ ).

- 
- [1] M. Gajdoš, K. Hummer, G. Kresse, J. Furthmüller, and F. Bechstedt, Linear optical properties in the projector-augmented wave methodology, *Phys. Rev. B* **73**, 045112 (2006).
  - [2] S. L. Adler, Quantum theory of the dielectric constant in real solids, *Phys. Rev.* **126**, 413 (1962).
  - [3] N. Wiser, Dielectric constant with local field effects included, *Phys. Rev.* **129**, 62 (1963).
  - [4] M. Dresselhaus *et al.*, Solid state physics part ii optical properties of solids, Lecture Notes (Massachusetts Institute of Technology, Cambridge, MA) **17**, 15 (2001).
  - [5] L. Yu and A. Zunger, Identification of potential photovoltaic absorbers based on first-principles spectroscopic screening of materials, *Phys. Rev. Lett.* **108**, 068701 (2012).
  - [6] T. Tiedje, E. Yablonovitch, G. D. Cody, and B. G. Brooks, Limiting efficiency of silicon solar cells, *IEEE Transactions on electron devices* **31**, 711 (1984).
